# Supplementary material for: Meridional composite pulses for low-field magnetic resonance
Source: arXiv:2206.12025 source file (2022-06-24)
Supplement: Supplementary file 1 [file SM.pdf]

# Meridional Composite Pulses for Low-field Magnetic Resonance

### Supplemental Material

**Sven Bodenstedt[a], Morgan W. Mitchell[a,b], Michael C. D. Tayler[a,*]**

[a] *ICFO-Institut de Ciències Fotòniques, The Barcelona Institute of Science and Technology, 08860 Castelldefels (Barcelona), Spain.*

[b] *ICREA – Institució Catalana de Recerca i Estudis Avançats, 08010 Barcelona, Spain.*

[*] *Corresponding author. Email: michael dot tayler at icfo dot eu*

## Contents

S.1 BURP Flip-Angle Coefficients ....... 2
S.2 Meridional Plane Angles for Discrete BURPs ....... 3
S.3 Pulse Hardware Calibration ....... 4

## S.1 BURP Flip-Angle Coefficients

| | Pulse | | | |
|---|---|---|---|---|
| | I-BURP-1 | I-BURP-2 | E-BURP-1 | E-BURP-2 |
| $a_0$ | +3.142 | +3.142 | +1.445 | +1.634 |
| $a_1$ | +0.740 | +0.790 | +0.890 | +0.910 |
| $a_2$ | −0.100 | +0.000 | −0.510 | +0.225 |
| $a_3$ | −0.307 | −0.410 | −0.083 | −0.437 |
| $a_4$ | +0.030 | −0.048 | +0.035 | −0.030 |
| $a_5$ | −0.006 | +0.020 | +0.006 | +0.006 |
| $a_6$ | −0.007 | +0.020 | +0.007 | +0.002 |
| $b_0$ | −1.123 | −1.143 | −0.852 | −0.881 |
| $b_1$ | +1.520 | +0.710 | +0.400 | +0.120 |
| $b_2$ | −0.500 | +0.695 | +0.710 | +0.895 |
| $b_3$ | +0.103 | −0.103 | −0.247 | −0.003 |
| $b_4$ | +0.008 | −0.117 | −0.015 | −0.102 |
| $b_5$ | −0.016 | −0.044 | −0.006 | −0.016 |
| $b_6$ | +0.008 | −0.005 | +0.007 | −0.012 |

Table 1: Fourier coefficients for the flip angle, $\beta(t)$, of various Broadband Uniform excitation Pure-Phase (BURP[1]) pulses, as defined in Eq. (5) of the main paper. Within the passband of the pulses, $\beta(\tau_p) \equiv a_0$, therefore for an inversion (I-BURP) pulse $a_0 = \pi$, while for an excitation (E-BURP) pulse $a_0 \approx \pi/2$.

## S.2 Meridional Plane Angles for Discrete BURPs

Here we list $\phi_j$ angles obtained upon discretization of the I-BURP-1 pulse into $N$ equal-length sections, according to Eq. (6) of the main manuscript. The chosen values of $N$ are equal to those used in Figure 4.

| | Pulse length parameter $N$ | | | | | | | | |
|---|---|---|---|---|---|---|---|---|---|
| | 10 | 12 | 14 | 16 | 18 | 20 | 40 | | 40 |
| $\phi_1$ | +17.85 | +12.04 | +8.59 | +6.44 | +5.03 | +4.06 | +1.30 | $\phi_{21}$ | +7.63 |
| $\phi_2$ | +43.86 | +35.71 | +27.89 | +21.81 | +17.24 | +13.78 | +2.76 | $\phi_{22}$ | +11.30 |
| $\phi_3$ | −13.89 | +21.14 | +29.52 | +28.72 | +25.48 | +22.01 | +5.50 | $\phi_{23}$ | +13.33 |
| $\phi_4$ | −107.01 | −52.20 | −8.86 | +11.92 | +19.95 | +21.85 | +8.29 | $\phi_{24}$ | +14.14 |
| $\phi_5$ | −35.13 | −90.39 | −68.11 | −31.31 | −6.54 | +7.17 | +10.40 | $\phi_{25}$ | +14.28 |
| $\phi_6$ | +46.40 | −20.62 | −70.97 | −69.81 | −44.47 | −21.06 | +11.61 | $\phi_{26}$ | +14.01 |
| $\phi_7$ | +55.98 | +36.93 | −12.38 | −54.66 | −64.52 | −50.27 | +11.71 | $\phi_{27}$ | +13.79 |
| $\phi_8$ | +71.01 | +47.04 | +30.28 | −7.42 | −42.19 | −56.75 | +10.14 | $\phi_{28}$ | +13.83 |
| $\phi_9$ | +74.36 | +49.82 | +40.48 | +25.43 | −4.30 | −32.88 | +6.45 | $\phi_{29}$ | +14.76 |
| $\phi_{10}$ | +26.57 | +67.53 | +39.86 | +35.24 | +21.77 | −2.25 | +0.72 | $\phi_{30}$ | +16.66 |
| $\phi_{11}$ | | +54.73 | +50.82 | +34.73 | +30.98 | +18.93 | −6.52 | $\phi_{31}$ | +18.95 |
| $\phi_{12}$ | | +18.26 | +58.49 | +38.38 | +31.22 | +27.47 | −14.55 | $\phi_{32}$ | +20.65 |
| $\phi_{13}$ | | | +41.08 | +50.17 | +31.44 | +28.36 | −22.28 | $\phi_{33}$ | +21.07 |
| $\phi_{14}$ | | | +13.30 | +48.59 | +39.56 | +27.62 | −27.98 | $\phi_{34}$ | +20.08 |
| $\phi_{15}$ | | | | +31.63 | +46.36 | +31.42 | −29.79 | $\phi_{35}$ | +18.00 |
| $\phi_{16}$ | | | | +10.14 | +40.05 | +39.60 | −26.95 | $\phi_{36}$ | +15.20 |
| $\phi_{17}$ | | | | | +24.92 | +41.15 | −20.47 | $\phi_{37}$ | +11.87 |
| $\phi_{18}$ | | | | | +8.02 | +33.20 | −12.41 | $\phi_{38}$ | +8.17 |
| $\phi_{19}$ | | | | | | +20.04 | −4.53 | $\phi_{39}$ | +4.56 |
| $\phi_{20}$ | | | | | | +6.53 | +2.28 | $\phi_{40}$ | +1.96 |

Table 2: Angles for band-pass-inversion meridional composite pulses based on uniform discretization of I-BURP-1. All angles are given in degrees, rounded to two decimal places.

## S.3 Pulse Hardware Calibration

The electronic circuit shown in Fig. 3a of the main article is used to vary the current applied to the X field coil. Here we confirm the linearity between the output voltage of the digital-to-analog converter (dac, $V_{\mathrm{dac}}$) and the magnetic field produced at the coils ($B_X$).

The voltage produced by the dac is nominally

$$V_{\mathrm{dac}} = \left(\frac{v}{4096}\right) 3.3 \text{ volts}\,, \tag{1}$$

where $0 \leq v \leq 4095$ is an integer sent to the dac software register during the pulse program.

The voltage $V_{\mathrm{dac}}$ is connected to the non-inverting input of the L272M operational amplifier. The amplifier's output is fed back to the inverting input via a potential divider circuit of resistors $R_1$ and $R_2$, to scale the output voltage, according to

$$V_{\mathrm{out}} = V_{\mathrm{dac}} \left(1 + \frac{R_1}{R_2}\right)\,. \tag{2}$$

In the present work, resistances $R_1 = 47\,\mathrm{k\Omega}$ and $R_2 = 22\,\mathrm{k\Omega}$ are used, so that the amplifier gain gives a maximum output voltage of approximately 10 V. This is close to the maximum supply voltage limit of the H-bridge module, 11 V:

$$V_{\mathrm{out}} = v \times 2.53 \text{ mV}\,. \tag{3}$$

The voltage $V_{\mathrm{out}}$ is then applied across the coils via the H bridge circuit. We use the series resistance, $R_3$, and field-to-current ratio of the X coil, $\partial B_X/\partial I = 81\,\mathrm{\mu T\,A^{-1}}$, to write the magnetic field supplied:

$$B_X = \pm\left(\frac{V_{\mathrm{out}}}{R_3}\right)\left(\frac{\partial B_X}{\partial I}\right) = \left(\frac{1\,\Omega}{R_3}\right) v \times 205\,\mathrm{nT}\,. \tag{4}$$

The linear relation described in Equation 4 is experimentally verified by measuring the precession frequency of polarized $^1$H spins in a sample located at the coil center. The $^1$H spins are initially oriented along the $z$ axis and rotated in the $yz$ plane upon applying the field $B_X$ for a time duration $\tau_p$. Then follows spin precession under a magnetic field $B_Z = 0.47\,\mathrm{\mu T}$ to produce an observable nuclear spin induction signal at a Larmor frequency of 20 Hz. The amplitude of the signal follows a dependence

$$s(t, \tau_p) = s_0 \sin(\gamma_H B_X \tau_p) \cos(\gamma_H B_Z t)\,, \tag{5}$$

which we use to fit $B_X$. Fitted values of $\gamma_H B_X/(2\pi)$ (in Hz) from the experimental signals are plotted against $v$ in Figure 1. Datasets plotted in Figures 1a and 1b, respectively, are results for two values of series resistance ($R_3 = 8.8\,\Omega$ and $69\,\Omega$). These both demonstrate good linearity and range control of the dc fields.

# References


[1] H. Geen and R. Freeman, Band-selective radiofrequency pulses, *J. Magn. Reson (1969)* **93**, 93–141 (1991).

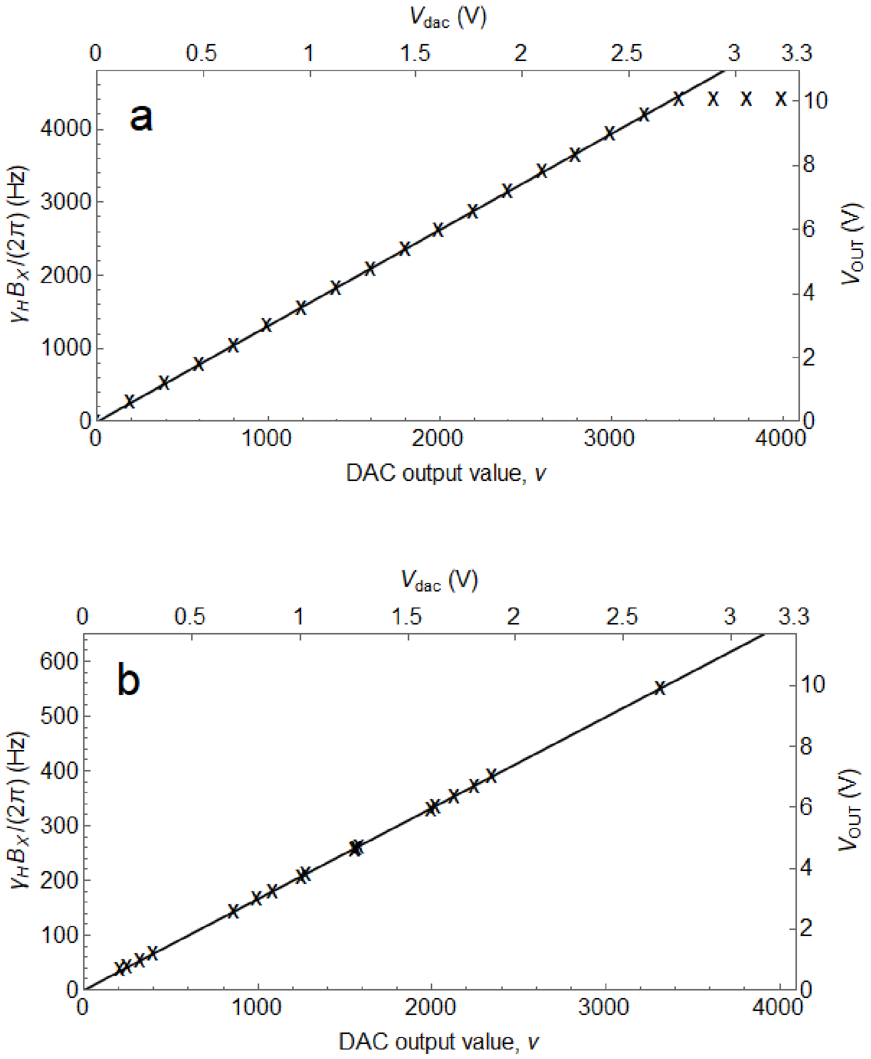


Figure 1: Spin precession frequencies vs. 12-bit DAC index values $0 \le v \le 4095$ for resistances (a) $R_3 = 8.8\,\Omega$ and (b) $R_3 = 69\,\Omega$. In (b), plotted values of $v$ correspond to those for an I-BURP-1 pulse with discretization number $N = 18$.
